# Supplementary material for: Functionalized few-layer silicene nanosheets: density functional theory on stability, structural, and electronic properties
Source: arXiv:2111.07694 source file (2021-11-15)
Supplement: Supplementary file 1 [file suppinfo.tex]

%%%%%%%%%%%%%%%%%%%%%%%%%%%%%%%%%%%%%%%%%%%%%%%%%%%%%%%%%%%%%%%%%%%%%
%% The same is true for Supporting Information, which should use the
%% suppinfo environment.
%%%%%%%%%%%%%%%%%%%%%%%%%%%%%%%%%%%%%%%%%%%%%%%%%%%%%%%%%%%%%%%%%%%%%
\begin{suppinfo}

\end{suppinfo}
